# Supplementary material for: MuTual: A Dataset for Multi-Turn Dialogue Reasoning
Source: arXiv:2004.04494 source file (2020-04-09)
Supplement: Supplementary file 1 [file appendix.tex]

\clearpage

\begin{appendices}

\section{Samples}
%895, 18, 94, 4224, 1115, 7699, 2888 todo
\begin{figure}[h!]
    \centering
    \includegraphics[width=0.5\textwidth]{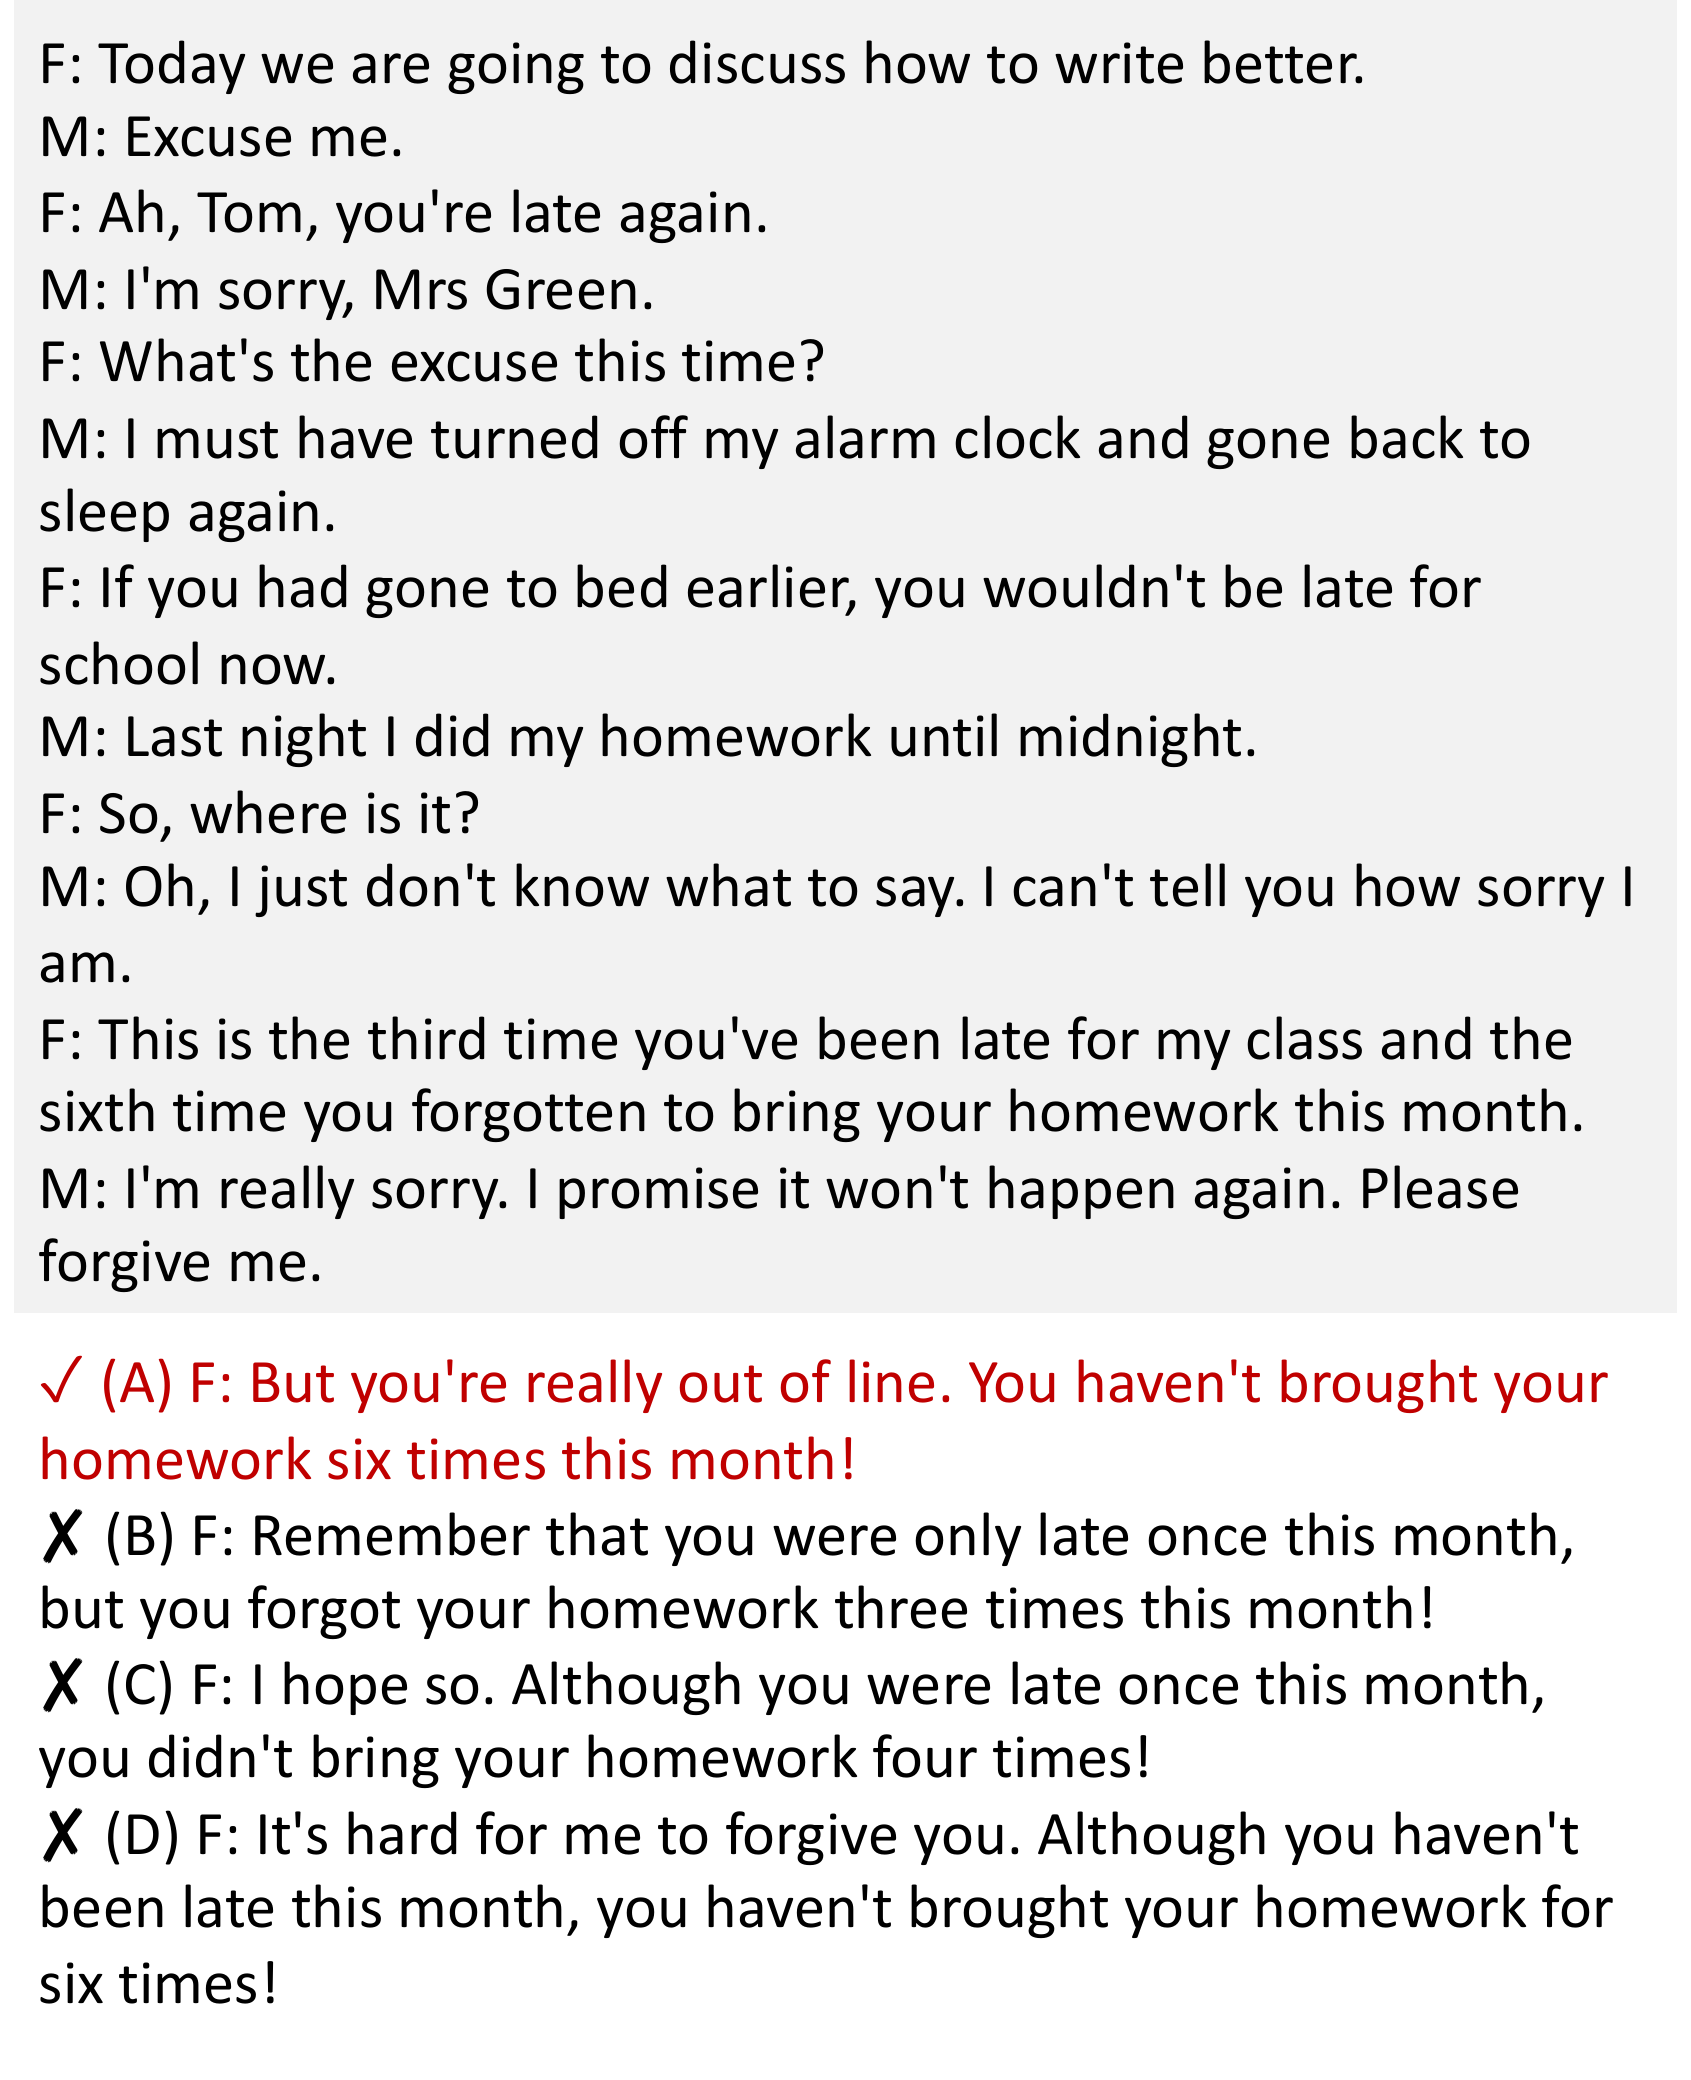}
    \includegraphics[width=0.5\textwidth]{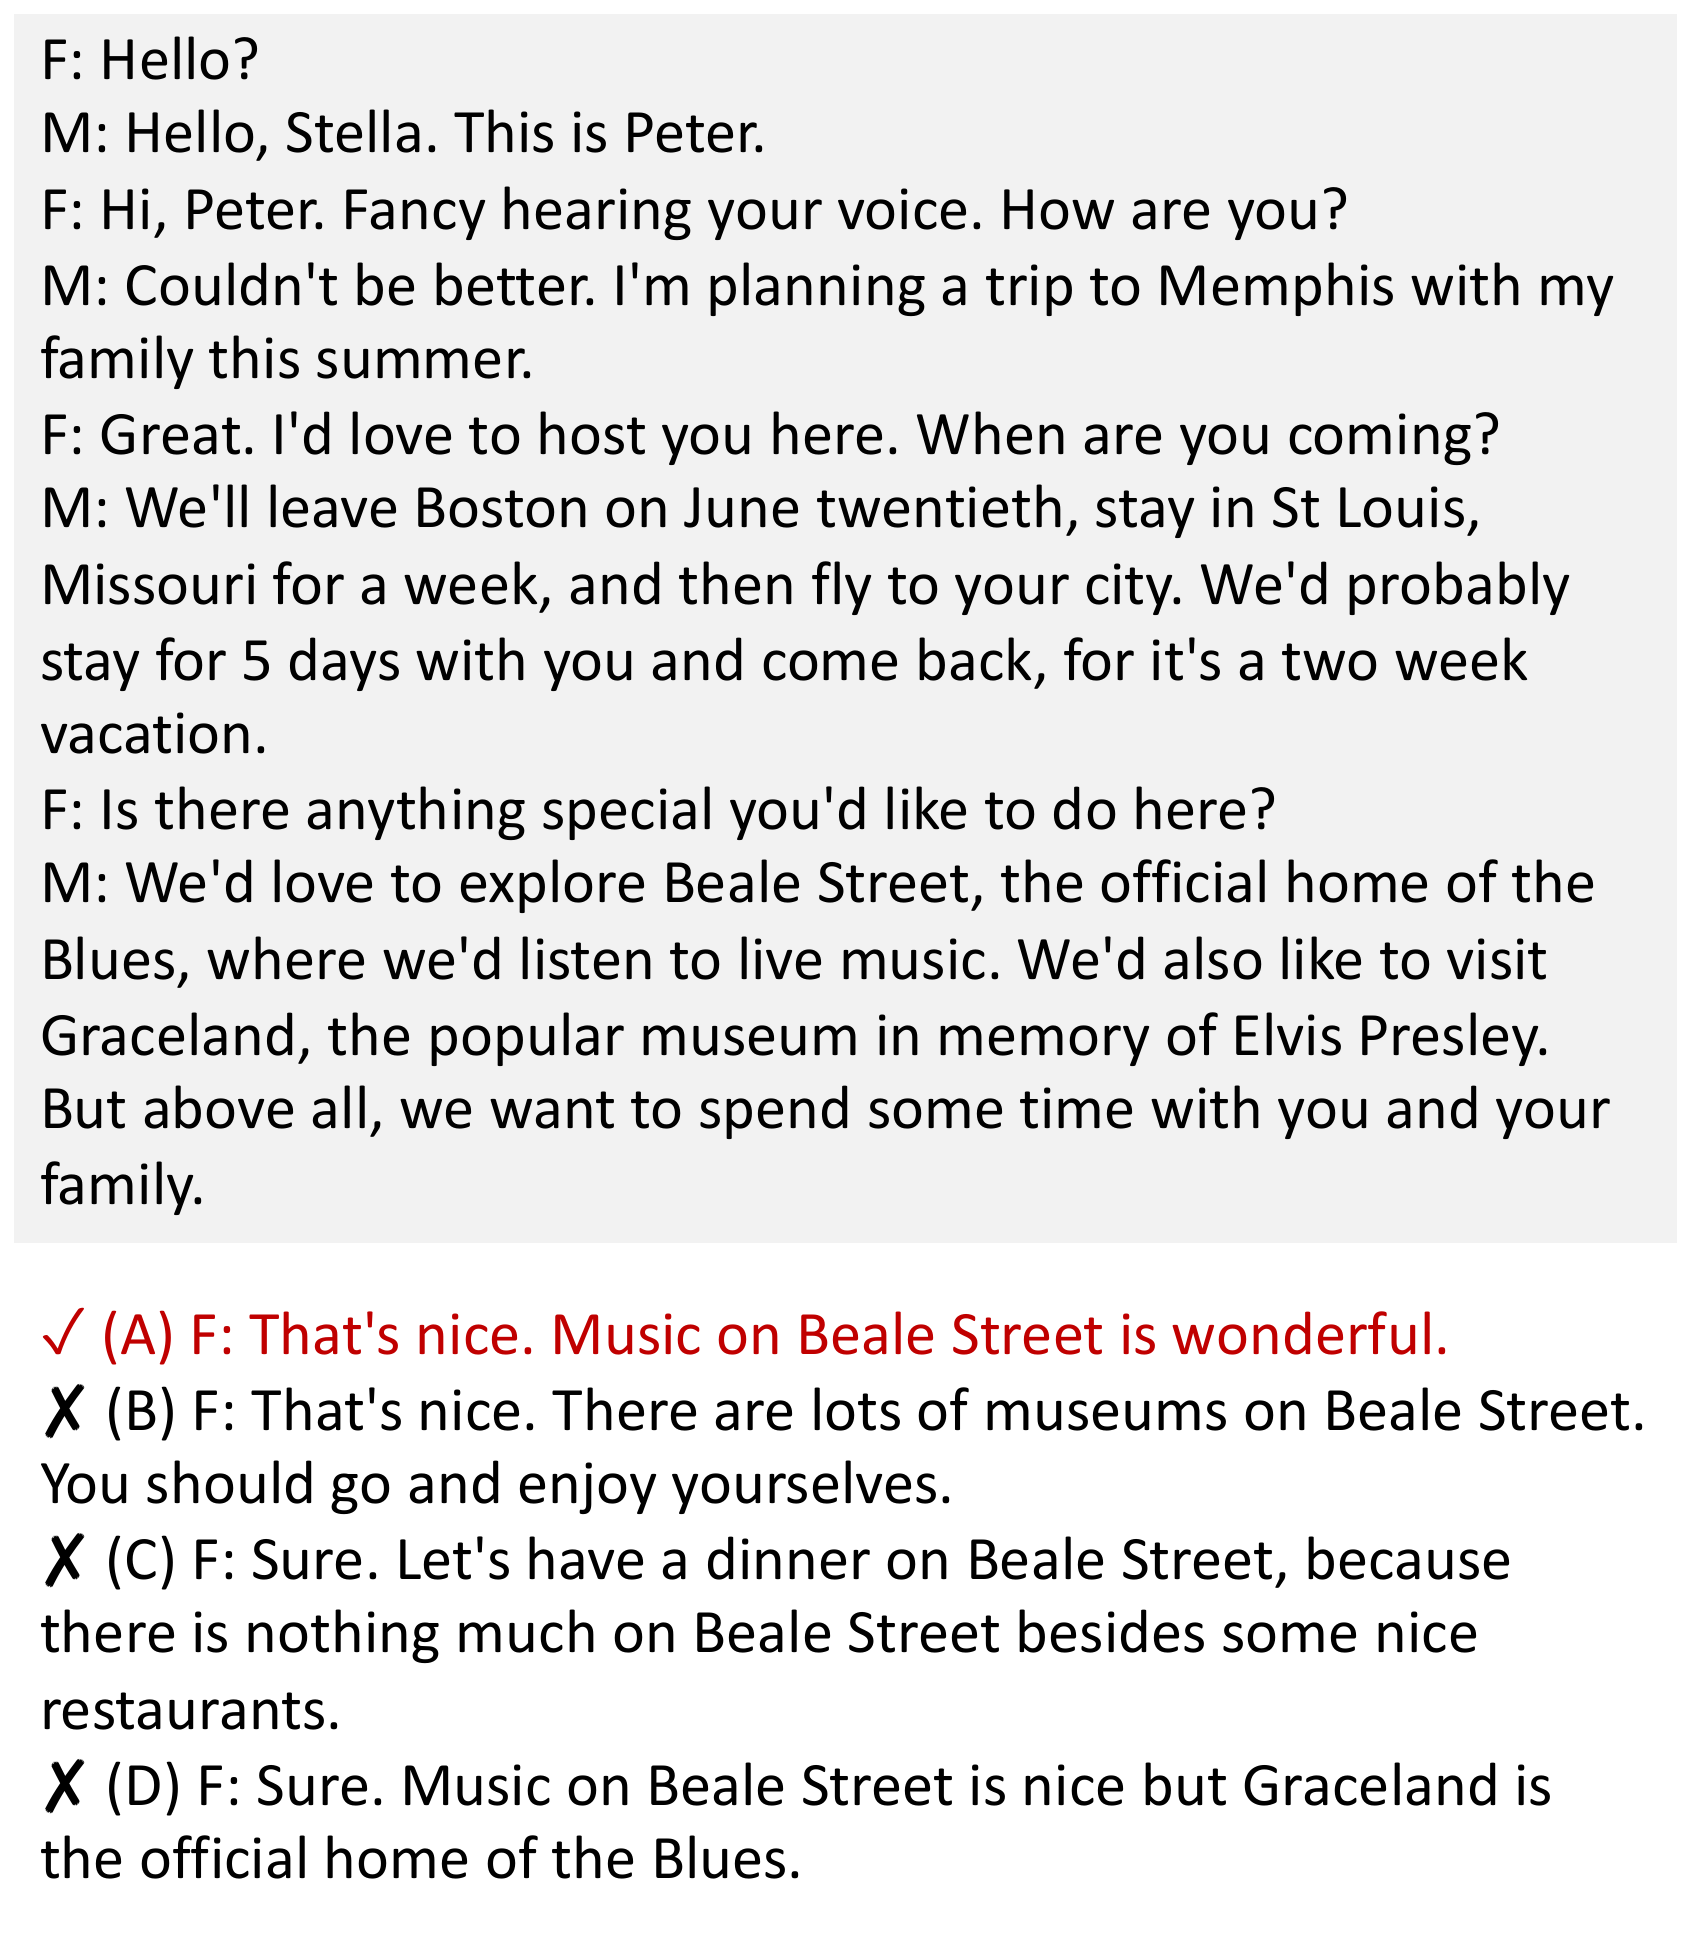}
\end{figure}

\begin{figure}[t!]
    \centering
    \includegraphics[width=0.5\textwidth]{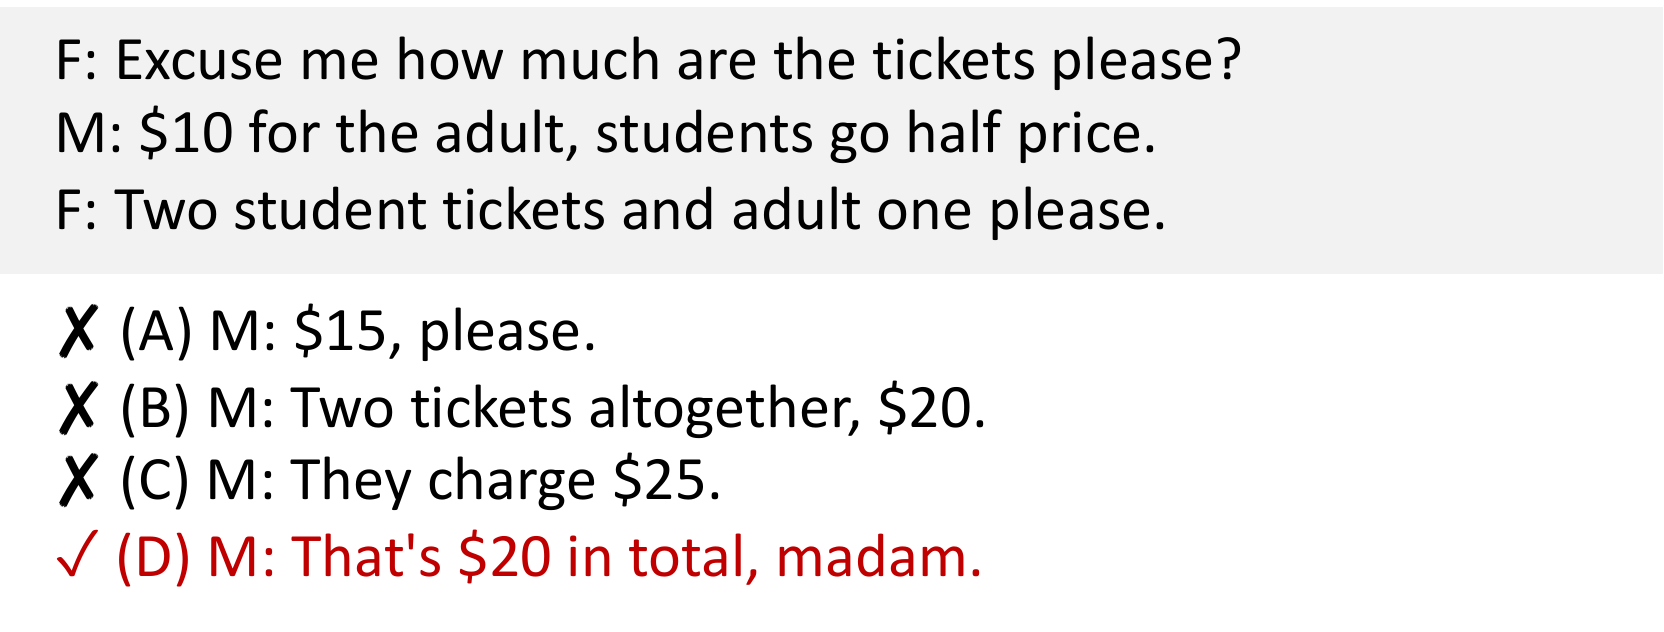}
    \includegraphics[width=0.5\textwidth]{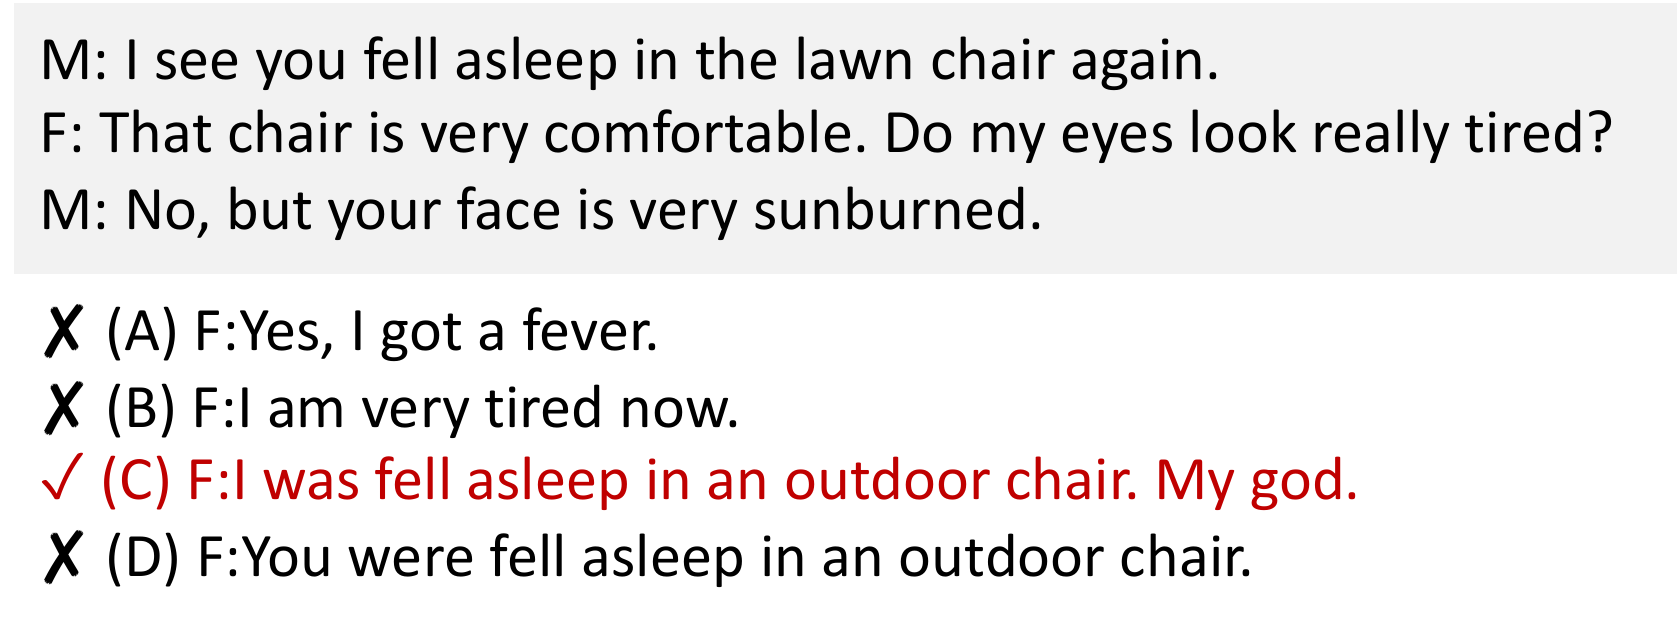}
    \includegraphics[width=0.5\textwidth]{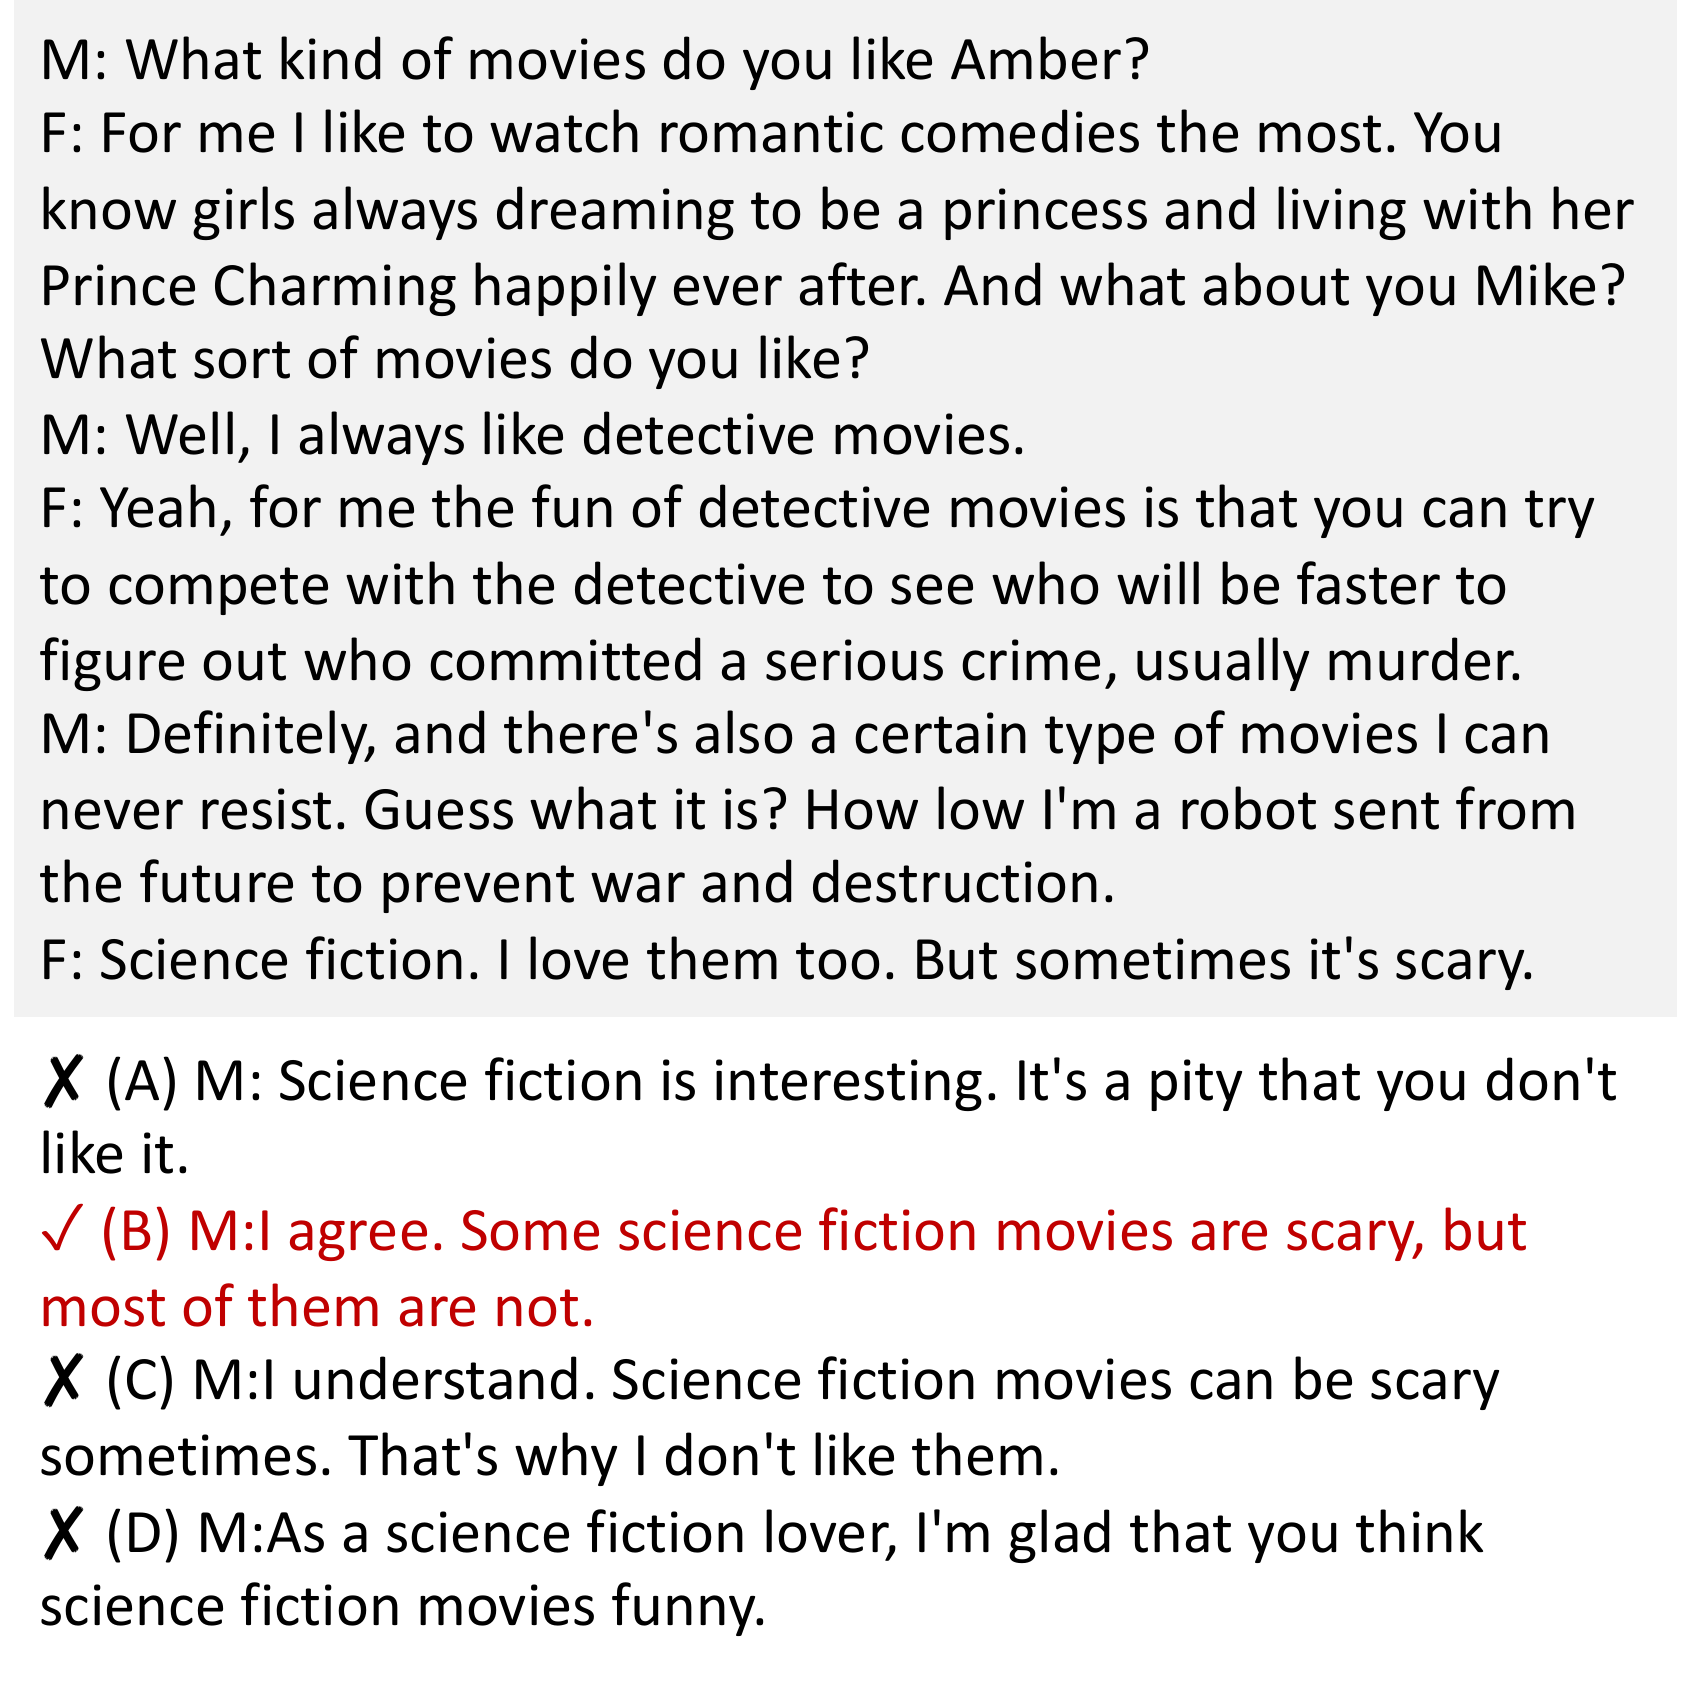}
    \includegraphics[width=0.5\textwidth]{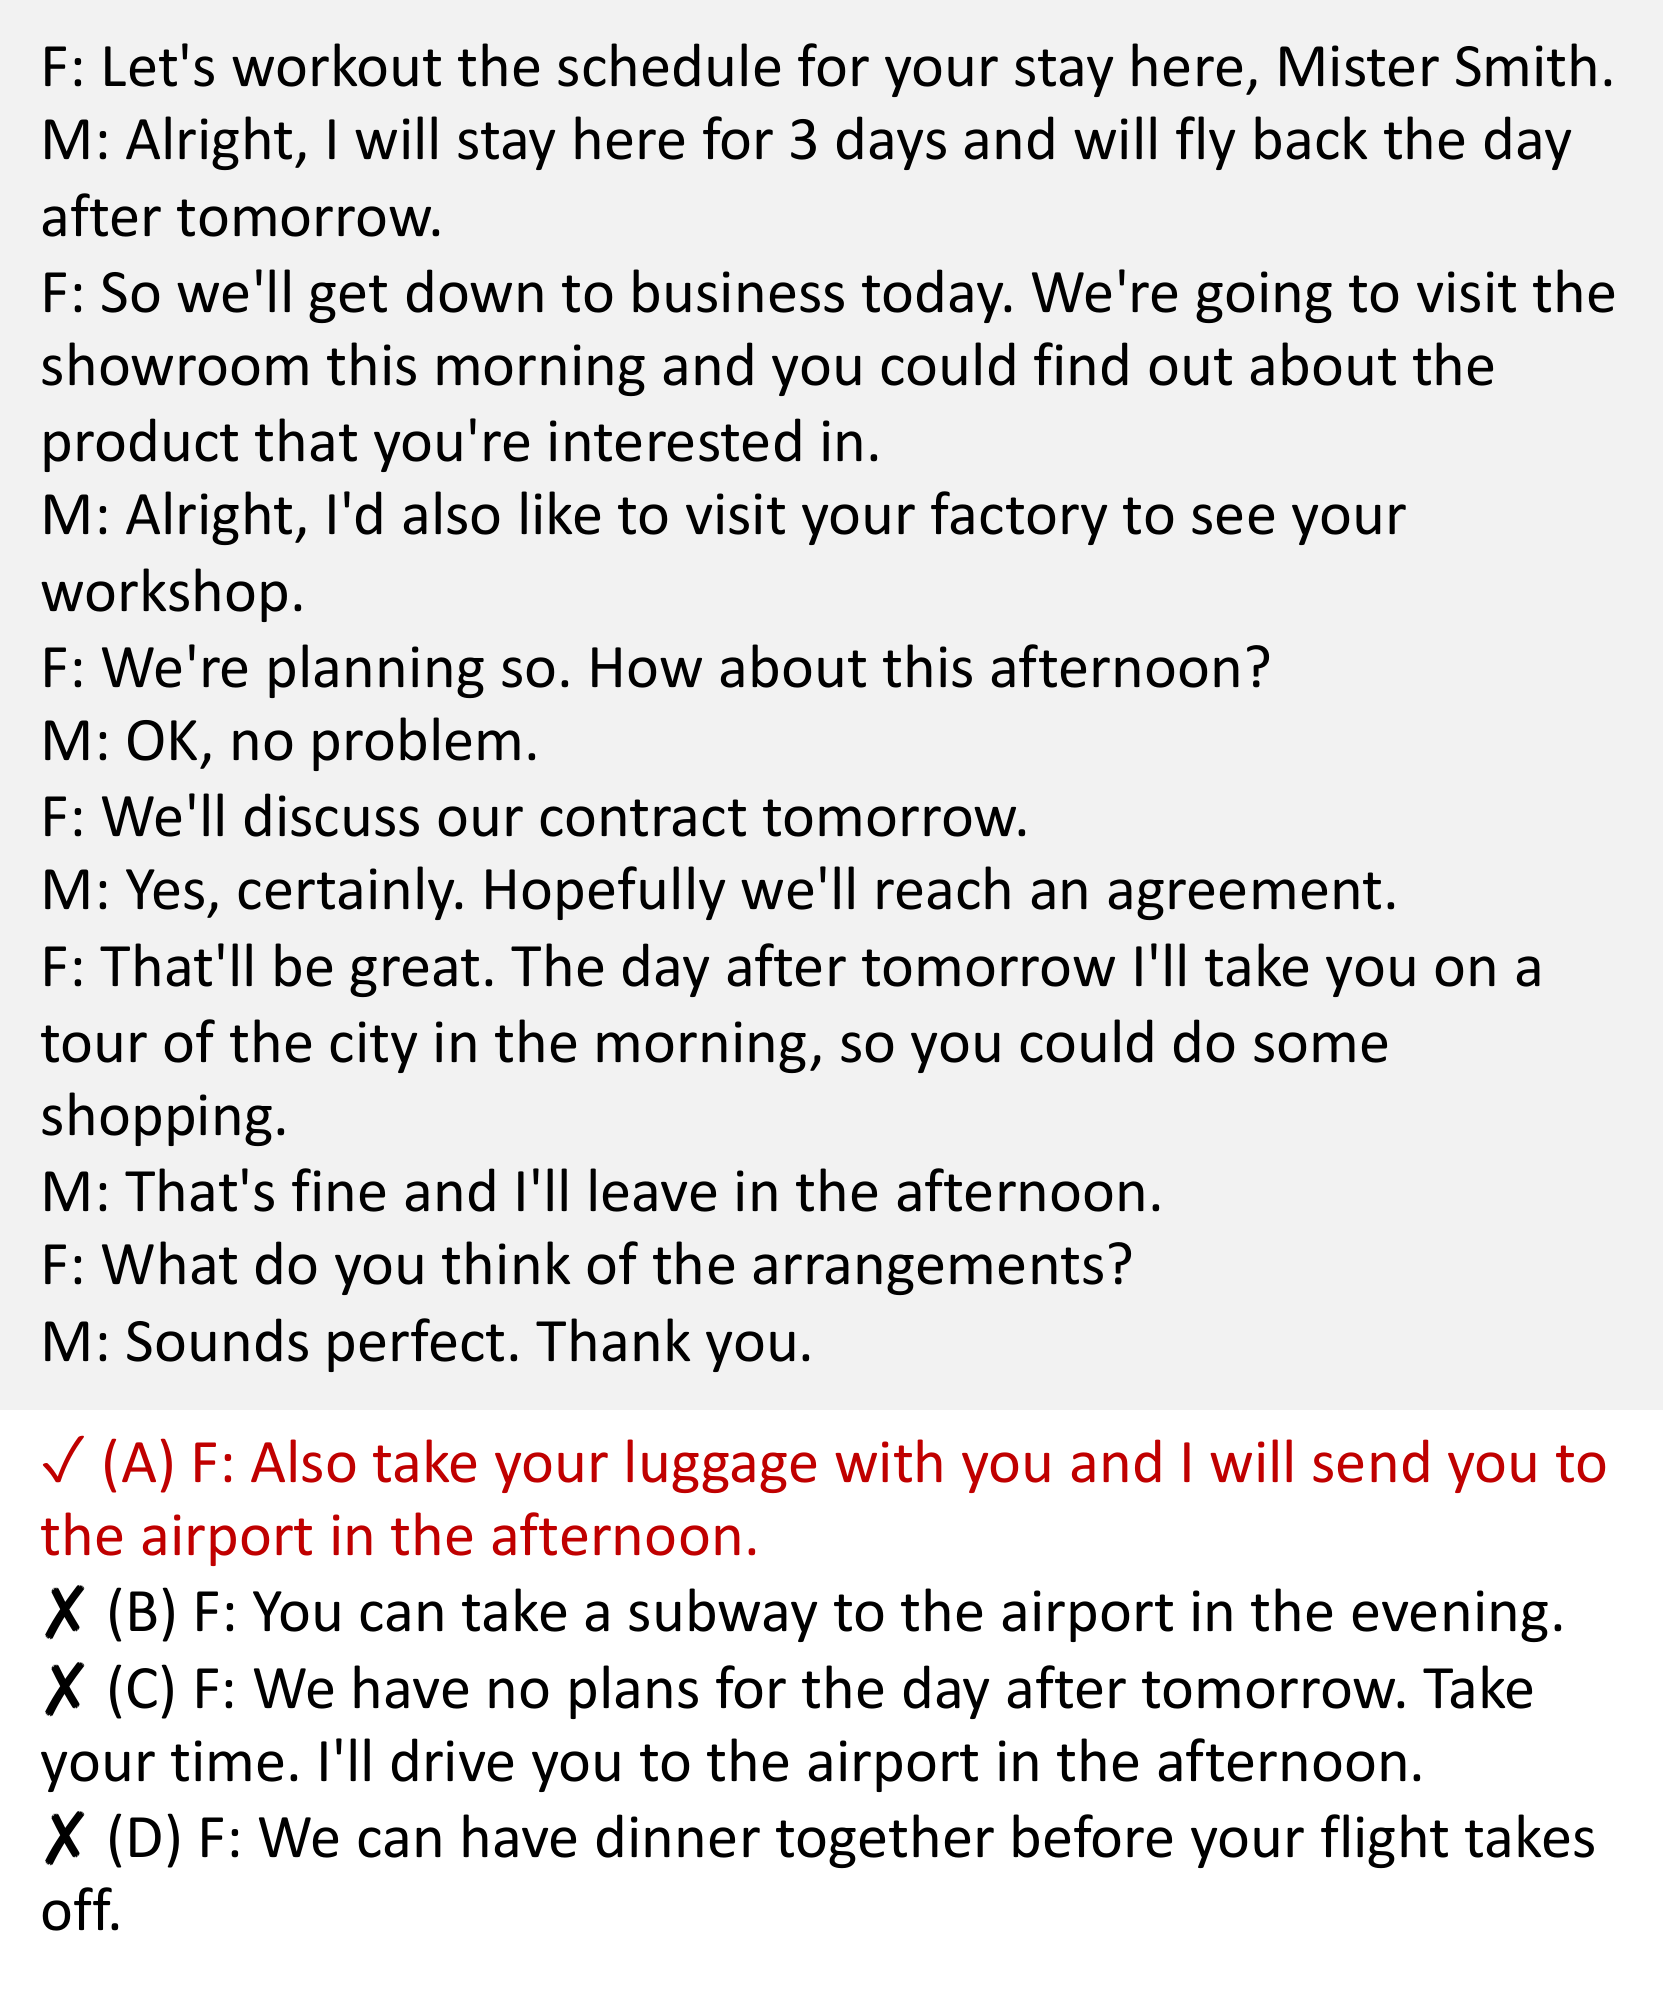}
\end{figure}

\section{Implementation Details}

% We keep the speaker identification (i.e., ``F:'', ``M:''), and convert number words to numeric digits

For SMN and DAM, we use the implementation from the original paper and retrain them on MuTual and MuTual$^{\text{plus}}$. One exception is that we use the 100-dimensional Glove word embedding to replace the original 100-dimensional ubuntu word embedding as embedding initialization. 

For all the experiments of BERT, BERT-MC, RoBERTa, RoBERTa-MC, GPT-2 and GPT-2-FT, we use the huggingface implementation. We fine-tune models for 5 epochs with a learning rate of 1e-5. The batch size is set as 16.

\end{appendices}
